# Supplementary material for: The Silent Cost of Conversation History in LLM Reasoning
Source: arXiv:2611.20071 source file (2026-11-25)
Supplement: Supplementary file 1 [file supp_adwin_replay.tex]

frozen (historical ADWIN) & 0/180000 & 0 \\
corrected ADWIN & 5/180000 & 0 \\
CUSUM for CS/SS & 5/180000 & 0 \\
