# Supplementary material for: The Silent Cost of Conversation History in LLM Reasoning
Source: arXiv:2611.20071 source file (2026-11-25)
Supplement: Supplementary file 2 [file supp_adwin_v_power.tex]

0.1 & 0.00 & 0.00 & 0.00 & 0.00 \\
0.2 & 0.00 & 0.00 & 0.00 & 0.00 \\
0.3 & 0.00 & 0.00 & 0.00 & 0.00 \\
0.4 & 0.03 & 0.01 & 0.00 & 0.00 \\
0.5 & 0.19 & 0.07 & 0.04 & 0.00 \\
0.6 & 0.61 & 0.73 & 0.78 & 0.93 \\
