# Supplementary material for: The Silent Cost of Conversation History in LLM Reasoning
Source: arXiv:2611.20071 source file (2026-11-25)
Supplement: Supplementary file 3 [file supp_aggregated.tex]

10 & CQ & cusum & 71 (+3) & 64 (+13) & 49 (+15) & -- & -- \\
10 & CQ & page-hinkley & 75 (+7) & 69 (+18) & 53 (+19) & -- & -- \\
10 & LS & cusum & 68 (+0) & 64 (+13) & 62 (+28) & -- & -- \\
10 & LS & page-hinkley & 71 (+3) & 68 (+17) & -- & -- & -- \\
10 & ES & cusum & 77 (+9) & 63 (+12) & 53 (+19) & -- & -- \\
10 & ES & page-hinkley & 75 (+7) & 63 (+12) & 52 (+18) & -- & -- \\
20 & CQ & cusum & 71 (+3) & 67 (+16) & 54 (+20) & -- & -- \\
20 & CQ & page-hinkley & 74 (+6) & 69 (+18) & 55 (+21) & -- & -- \\
20 & LS & cusum & 68 (+0) & 67 (+16) & 63 (+29) & -- & -- \\
20 & LS & page-hinkley & 69 (+1) & 68 (+17) & 65 (+31) & -- & -- \\
20 & ES & cusum & 81 (+13) & 68 (+17) & 56 (+22) & -- & -- \\
20 & ES & page-hinkley & 79 (+11) & 67 (+16) & 55 (+21) & -- & -- \\
30 & CQ & cusum & 78 (+10) & 72 (+21) & 59 (+25) & -- & -- \\
30 & CQ & page-hinkley & 75 (+7) & 71 (+20) & 57 (+23) & -- & -- \\
30 & LS & cusum & 69 (+1) & 68 (+17) & 68 (+34) & -- & -- \\
30 & LS & page-hinkley & 71 (+3) & 70 (+19) & 70 (+36) & -- & -- \\
30 & ES & cusum & 85 (+17) & 69 (+18) & 62 (+28) & -- & -- \\
30 & ES & page-hinkley & 88 (+20) & 73 (+22) & 64 (+30) & -- & -- \\
