# Supplementary material for: The Silent Cost of Conversation History in LLM Reasoning
Source: arXiv:2611.20071 source file (2026-11-25)
Supplement: Supplementary file 4 [file supp_control_screen.tex]

10 & distribution based & 0.22 (0.08) & 0.06 (0.08) & 0.00 (0.00) \\
10 & proposal mapping & 0.22 (0.08) & 0.06 (0.08) & 0.22 (0.00) \\
10 & adwin all & 0.00 (0.00) & 0.00 (0.00) & 0.00 (0.00) \\
20 & distribution based & 0.00 (0.08) & 0.06 (0.08) & 0.00 (0.08) \\
20 & proposal mapping & 0.00 (0.08) & 0.22 (0.08) & 0.00 (0.00) \\
20 & adwin all & 0.00 (0.00) & 0.00 (0.00) & 0.00 (0.00) \\
30 & distribution based & 0.06 (0.08) & 0.17 (0.08) & 0.11 (0.08) \\
30 & proposal mapping & 0.06 (0.08) & 0.28 (0.08) & 0.00 (0.00) \\
30 & adwin all & 0.00 (0.00) & 0.00 (0.00) & 0.00 (0.00) \\
