# Supplementary material for: The Silent Cost of Conversation History in LLM Reasoning
Source: arXiv:2611.20071 source file (2026-11-25)
Supplement: Supplementary file 5 [file supp_early_signal.tex]

10 & 17/18 & 3/12 & 10 & 7/0/3 & 5/12 & 5/2/8 \\
20 & 18/18 & 3/12 & 10 & 7/1/2 & 4/12 & 5/1/8 \\
30 & 17/18 & 3/12 & 11 & 7/2/2 & 2/12 & 1/1/13 \\
