# Supplementary material for: The Silent Cost of Conversation History in LLM Reasoning
Source: arXiv:2611.20071 source file (2026-11-25)
Supplement: Supplementary file 6 [file supp_h1a.tex]

S1-a & CQ & -0.094 & 18 & $<$0.001 & 0.001 \\
S1-a & CS & -0.033 & 6 & 0.219 & 1.000 \\
S1-a & RS & 0.006 & 6 & 0.563 & 1.000 \\
S1-a & LS & -0.045 & 18 & 0.033 & 0.380 \\
S1-a & ES & -0.060 & 18 & $<$0.001 & 0.001 \\
S1-a & SS & -0.000 & 6 & 0.469 & 1.000 \\
S1-b & CQ & -0.039 & 18 & 0.068 & 0.611 \\
S1-b & CS & -0.125 & 6 & 0.078 & 0.625 \\
S1-b & RS & 0.250 & 5 & 0.875 & 1.000 \\
S1-b & LS & -0.006 & 18 & 0.378 & 1.000 \\
S1-b & ES & -0.033 & 18 & 0.029 & 0.380 \\
S1-b & SS & -0.008 & 6 & 0.016 & 0.266 \\
S2 & CQ & -0.072 & 18 & $<$0.001 & 0.003 \\
S2 & CS & -0.167 & 6 & 0.016 & 0.266 \\
S2 & RS & -0.208 & 6 & 0.125 & 0.875 \\
S2 & LS & -0.063 & 18 & 0.003 & 0.061 \\
S2 & ES & -0.047 & 18 & $<$0.001 & 0.008 \\
S2 & SS & -0.010 & 6 & 0.031 & 0.380 \\
S3-a & CQ & -0.161 & 18 & $<$0.001 & 0.005 \\
S3-a & CS & -0.161 & 6 & 0.016 & 0.266 \\
S3-a & RS & -0.017 & 5 & 0.500 & 1.000 \\
S3-a & LS & -0.043 & 18 & 0.058 & 0.577 \\
S3-a & ES & -0.104 & 18 & $<$0.001 & 0.017 \\
S3-a & SS & -0.012 & 6 & 0.016 & 0.266 \\
