# Supplementary material for: The Silent Cost of Conversation History in LLM Reasoning
Source: arXiv:2611.20071 source file (2026-11-25)
Supplement: Supplementary file 7 [file supp_h1b.tex]

S1-a & 0.033 & 6 & 0.938 & 1.000 \\
S1-b & 0.150 & 6 & 0.969 & 1.000 \\
S2 & 0.200 & 6 & 1.000 & 1.000 \\
S3-a & 0.225 & 6 & 1.000 & 1.000 \\
