# Supplementary material for: The Silent Cost of Conversation History in LLM Reasoning
Source: arXiv:2611.20071 source file (2026-11-25)
Supplement: Supplementary file 8 [file supp_hashes.tex]

Study 1 raw records & \texttt{e313f1ce59854d25\ldots} \\
Study 1 confirmatory assessment & \texttt{1be56fb6bb98e6f8\ldots} \\
Study 2 frozen mappings & \texttt{4ab2af3d7af6deff\ldots} \\
Study 2 main manifest & \texttt{5351be89f927e36d\ldots} \\
Study 2 Stage A record prefix & \texttt{5e1b66ccf791c0fa\ldots} \\
Study 2 analysis protocol & \texttt{684fecef7c29d29a\ldots} \\
Study 2 acquisition fingerprint & \texttt{e5a9895be395fa00\ldots} \\
