# Supplementary material for: The Silent Cost of Conversation History in LLM Reasoning
Source: arXiv:2611.20071 source file (2026-11-25)
Supplement: Supplementary file 9 [file supp_kdiv.tex]

Llama-4 Scout  & pilot, 100 turns & 0.38 & 1.00 & 0 \\
Llama-4 Scout  & 26 probe turns & 0.50 & 1.00 & 0 \\
Llama-4 Maverick  & 30 probe turns & 0.63 & 1.00 & 0 \\
Llama-4 Maverick & 30 probe turns & 0.70 & 1.00 & 0 \\
Llama-3 8B & 30 probe turns & 0.63 & 1.00 & 0 \\
Llama-3 70B & 30 probe turns & 1.00 & 0.97 & 0 \\
