# Supplementary material for: The Silent Cost of Conversation History in LLM Reasoning
Source: arXiv:2611.20071 source file (2026-11-25)
Supplement: Supplementary file 10 [file supp_ladder.tex]

1 & 2 & 1 & 0 & 0 \\
2 & 2 & 1 & 1 & 0 \\
3 & 2 & 2 & 1 & 0 \\
4 & 3 & 2 & 1 & 0 \\
5 & 3 & 2 & 1 & 1 \\
6 & 3 & 2 & 2 & 1 \\
7 & 4 & 2 & 2 & 1 \\
8 & 4 & 3 & 2 & 1 \\
9 & 5 & 3 & 2 & 1 \\
10 & 5 & 3 & 2 & 2 \\
11 & 6 & 3 & 2 & 2 \\
12 & 6 & 3 & 3 & 2 \\
13$^\dagger$ & 8 & 3 & 4 & 2 \\
14$^\dagger$ & 10 & 4 & 5 & 2 \\
