# Supplementary material for: The Silent Cost of Conversation History in LLM Reasoning
Source: arXiv:2611.20071 source file (2026-11-25)
Supplement: Supplementary file 11 [file supp_power_full.tex]

oracle & 10 & 1 & 0.5 & 0.4 \\
oracle & 10 & 3 & 0.3 & 0.2 \\
oracle & 10 & 6 & 0.2 & 0.2 \\
oracle & 10 & 18 & 0.1 & 0.1 \\
oracle & 20 & 1 & 0.5 & 0.4 \\
oracle & 20 & 3 & 0.3 & 0.3 \\
oracle & 20 & 6 & 0.2 & 0.2 \\
oracle & 20 & 18 & 0.1 & 0.1 \\
oracle & 30 & 1 & 0.5 & 0.4 \\
oracle & 30 & 3 & 0.3 & 0.3 \\
oracle & 30 & 6 & 0.2 & 0.2 \\
oracle & 30 & 18 & 0.1 & 0.1 \\
n36 & 10 & 1 & 0.5 & 0.4 \\
n36 & 10 & 3 & 0.3 & 0.3 \\
n36 & 10 & 6 & 0.2 & 0.2 \\
n36 & 10 & 18 & 0.1 & 0.1 \\
n36 & 20 & 1 & 0.5 & 0.5 \\
n36 & 20 & 3 & 0.3 & 0.3 \\
n36 & 20 & 6 & 0.2 & 0.2 \\
n36 & 20 & 18 & 0.1 & 0.1 \\
n36 & 30 & 1 & 0.6 & 0.4 \\
n36 & 30 & 3 & 0.3 & 0.3 \\
n36 & 30 & 6 & 0.3 & 0.2 \\
n36 & 30 & 18 & 0.2 & 0.1 \\
n12 & 10 & 1 & 0.5 & 0.4 \\
n12 & 10 & 3 & 0.3 & 0.3 \\
n12 & 10 & 6 & 0.2 & 0.2 \\
n12 & 10 & 18 & 0.1 & 0.1 \\
n12 & 20 & 1 & 0.5 & 0.5 \\
n12 & 20 & 3 & 0.3 & 0.3 \\
n12 & 20 & 6 & 0.2 & 0.2 \\
n12 & 20 & 18 & 0.1 & 0.1 \\
n12 & 30 & 1 & 0.6 & 0.5 \\
n12 & 30 & 3 & 0.4 & 0.3 \\
n12 & 30 & 6 & 0.3 & 0.2 \\
n12 & 30 & 18 & 0.2 & 0.1 \\
