# Supplementary material for: The Silent Cost of Conversation History in LLM Reasoning
Source: arXiv:2611.20071 source file (2026-11-25)
Supplement: Supplementary file 12 [file supp_stagea_monitoring.tex]

10 & distribution based & n/c & 0.00 & 0.00 & 0.02 & n/c & 0.00 \\
10 & proposal mapping & n/c & 0.00 & 0.00 & 0.02 & 0.00 & 0.00 \\
10 & adwin all & 0.00 & 0.00 & 0.00 & 0.00 & 0.00 & 0.00 \\
20 & distribution based & n/c & 0.00 & 0.00 & 0.00 & 0.02 & 0.00 \\
20 & proposal mapping & n/c & 0.00 & 0.00 & 0.00 & 0.00 & 0.00 \\
20 & adwin all & 0.00 & 0.00 & 0.00 & 0.00 & 0.00 & 0.00 \\
30 & distribution based & 0.02 & 0.11 & 0.00 & 0.00 & 0.00 & 0.00 \\
30 & proposal mapping & 0.02 & 0.00 & 0.00 & 0.00 & 0.02 & 0.00 \\
30 & adwin all & 0.00 & 0.00 & 0.00 & 0.00 & 0.00 & 0.00 \\
